# Supplementary material for: Resonance dynamics of DCO ($\widetilde{X}\,{}^2A'$) simulated with the dynamically pruned discrete variable representation (DP-DVR)
Source: arXiv:1802.07050 ancillary file (2018-05-08)
Supplement: Supplementary file 1 [file esi_DCO.pdf]

*Supplementary material for*  
**Resonance dynamics of DCO ( $\tilde{X}^2A'$ ) simulated with the  
dynamically pruned discrete variable representation  
(DP-DVR)**

Henrik R. Larsson    Jens Riedel    Jie Wei    Friedrich Temps    Bernd Hartke

Institut für Physikalische Chemie, Christian-Albrechts-Universität zu Kiel,  
Olshausenstraße 40  
24098 Kiel, Germany

Journal of Chemical Physics

**Contents**

|                                            |    |
|--------------------------------------------|----|
| i. Potential energy surfaces               | 2  |
| ii. Propagation times                      | 4  |
| iii. Diabatization of rovibrational states | 4  |
| iv. Kinetic energy release spectra         | 6  |
| v. Rovibrational CO product distributions  | 10 |

## i. Potential energy surfaces

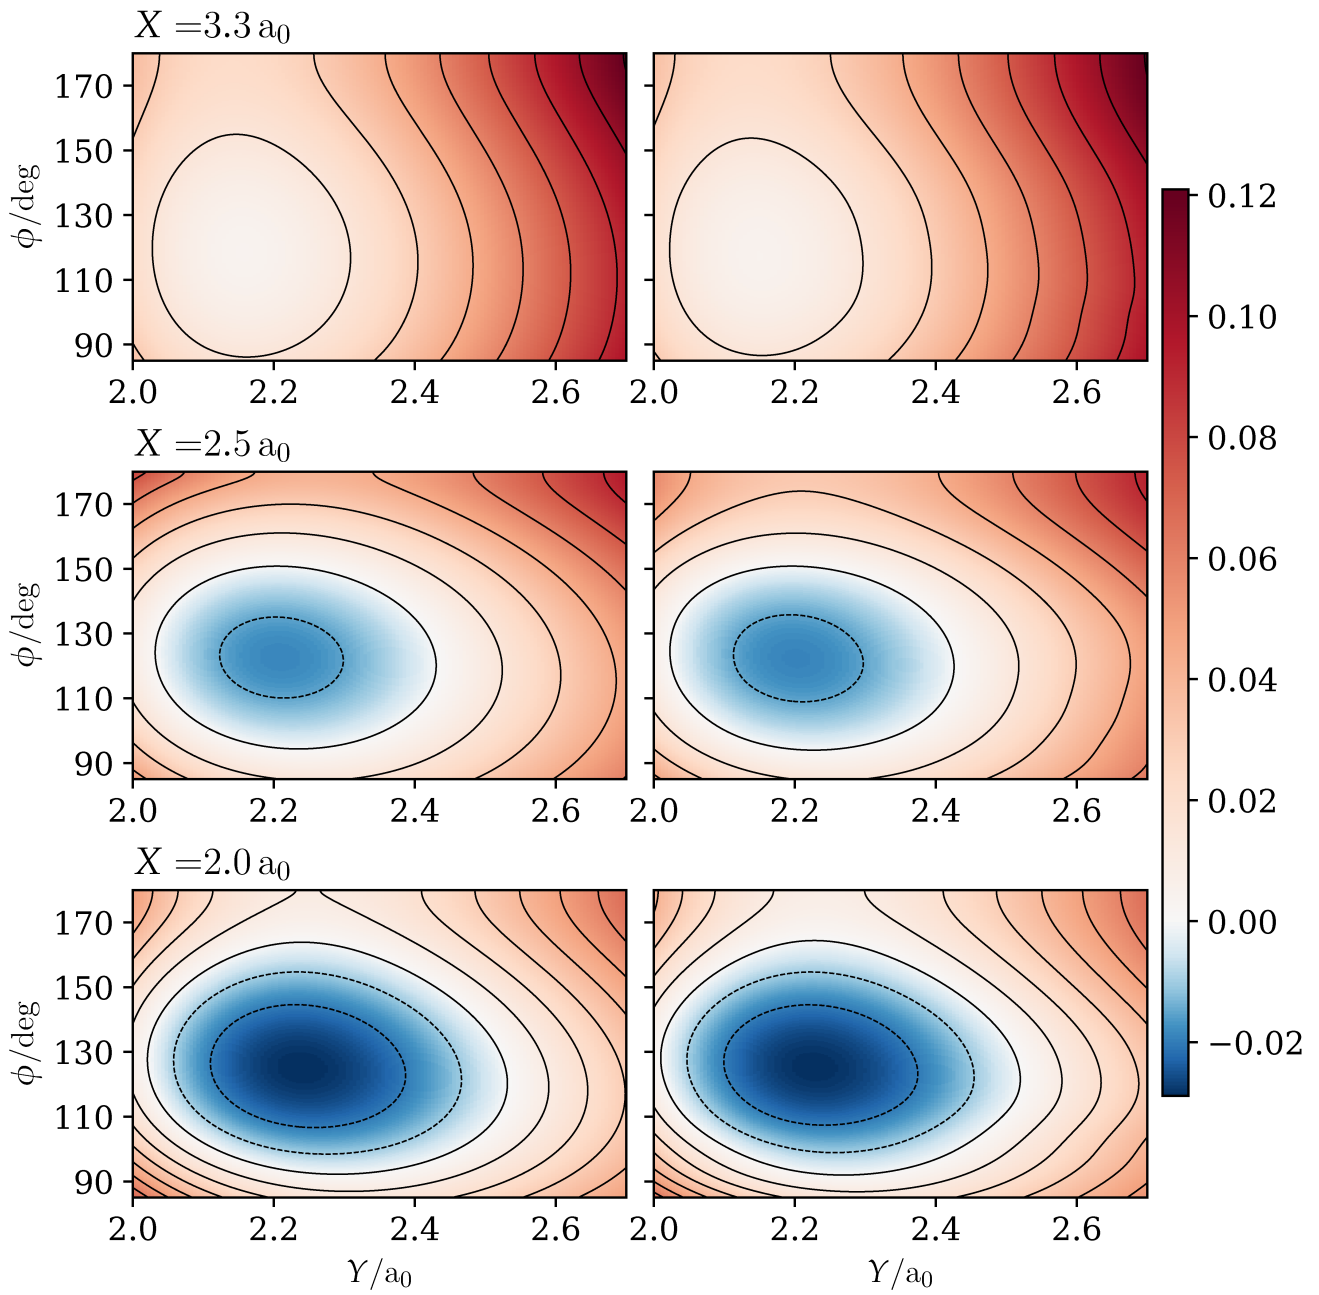

Figure i: Cuts through the WKS<sup>1,2</sup> (left) and SAG<sup>3</sup> (right) PES in Eckart bond coordinates.  $X$  is the D-CO distance,  $Y$  the DC=O distance and  $\phi$  the D-C=O bending angle. The values of the potential are given in Hartree.

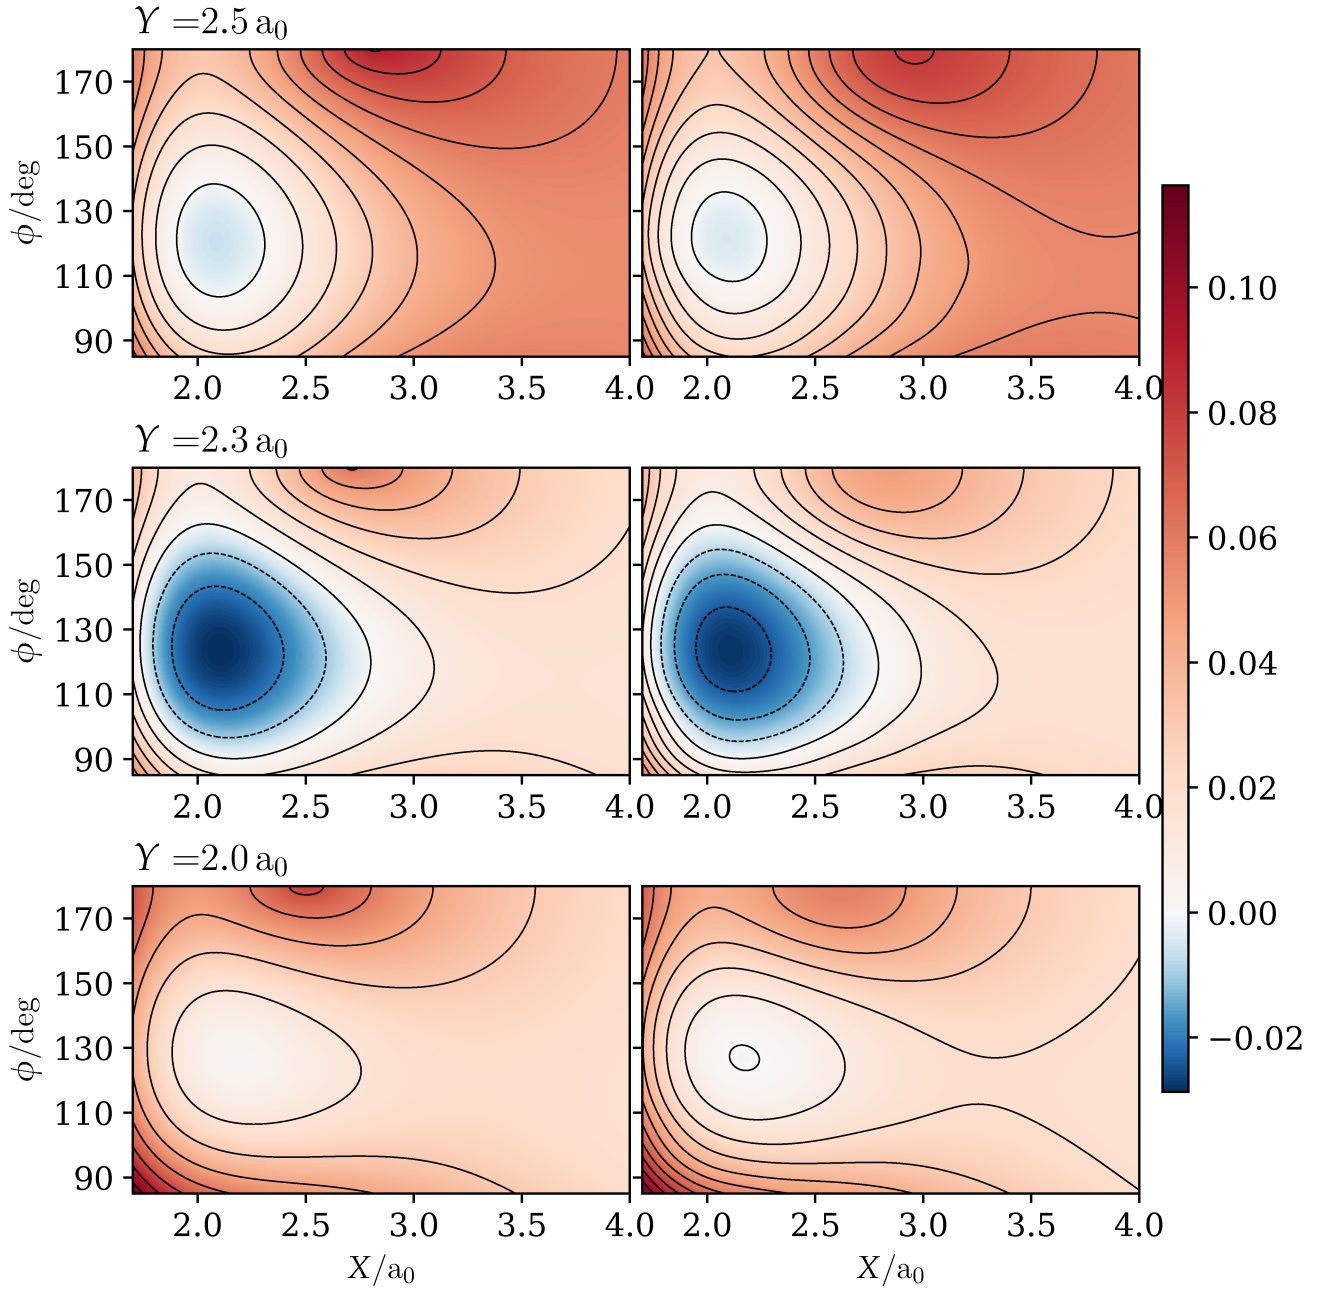

Figure ii: As Figure i but for cuts in  $Y$ .

## ii. Propagation times

Table i: Final propagation time  $t_{\text{end}}$  and norm of the wavefunction at that time for the simulations.

| label | WKS PES <sup>1,2</sup>     |      | SAG PES <sup>3</sup>       |       |
|-------|----------------------------|------|----------------------------|-------|
|       | $t_{\text{end}}/\text{ps}$ | norm | $t_{\text{end}}/\text{ps}$ | norm  |
| 034   | 27                         | 0.02 |                            |       |
| 042   | 27                         | 0.06 | 80                         | 0.02  |
| 222   | 24                         | 0.07 | 53                         | 0.07  |
| 050   | 175                        | 0.1  | 80                         | 0.005 |
| 132   | 89                         | 0.1  |                            |       |
| 230   | 80                         | 0.09 |                            |       |
| 027   | 22                         | 0.03 |                            |       |
| 140   | 80                         | 0.1  |                            |       |
| 043   | 27                         | 0.03 |                            |       |
| 223   | 30                         | 0.01 |                            |       |
| 051   | 60                         | 0.04 |                            |       |
| 133   | 30                         | 0.04 |                            |       |
| 231   | 28                         | 0.03 | 75                         | 0.08  |
| 141   | 27                         | 0.02 | 30                         | 0.1   |
| 321   | 30                         | 0.01 |                            |       |

## iii. Diabatization of rovibrational states

Although we tried many different diabatization schemes,<sup>4–7</sup> taking either the nonadiabatic coupling matrix elements explicitly into account or using other approaches solely based on the potential energy curves (diabatization by *ansatz*<sup>8,9</sup> or minimizing the curvature of the diabatic curves), we were not able to obtain useful (quasi-)diabatic states that have proper nodal patterns. Besides requiring the diabatization of *many* states (up to  $\sim 250$  are required for  $v_2 \leq 5$  and  $v_3 \leq 8$ ), the Hamiltonian introduces an “artificial” nonadiabatic coupling between the states. The coupling is artificially increased by the  $R$ -dependent part of the kinetic energy operator in Eq. (9) of the paper and by non-trivial changes in the potential. For example, an inspection of Fig. 4 shows that the adiabatic ground state does not strongly couple to other states and, of course, it does not change its character in terms of number of nodes. In other words, the adiabatic ground state can already be considered as a proper diabatic state that would suffice for further analysis. However, the shape of the ground-state wavefunction for different values of  $R$  differs drastically, because the cut of the potential changes significantly. For large  $R$ , the wavefunction has a prolate shape. With decreasing  $R$ , the function becomes more confined and the coordinates of the maximum describes a complicated path. The change of the shape introduces the “artificial” coupling such that the obtained diabatic states have a very complicated nodal pattern and are useless for a further analysis. This is shown in Figure iii.

One way to circumvent this “artificial” coupling is to remove the part from the nonadiabatic coupling that is due to the change in shape/location of the eigenstates, such that only the coupling remains that accounts for the mixing of the nodal pattern. This is similar to the procedure suggested by Esry and Sadeghpour.<sup>10</sup> It can be easily done for the  $R$ -dependent part of the kinetic energy operator. For the potential, this is much more difficult. We tried different  $R$ -dependent coordinate transforms trying to retain the shape of the ground state. This gave no satisfactory results for all  $R$  values because the changes in the potential are too complicated. Especially, an affine coordinate transformation does not suffice.

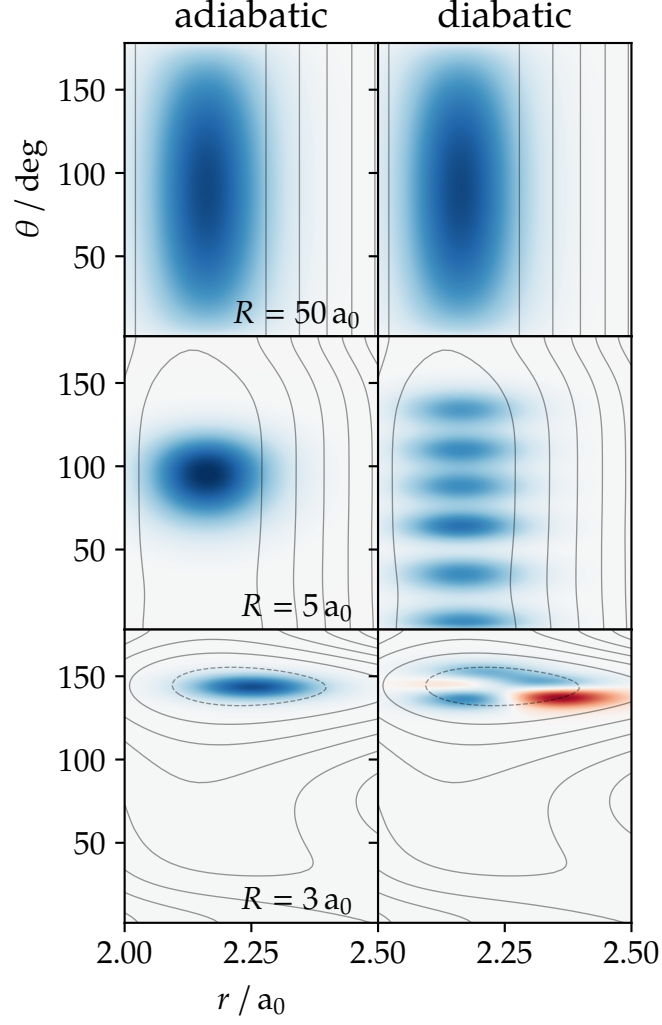

Figure iii: First adiabatic and diabatic state of the CO vibrational problem for different D–CO distances  $R$  in Jacobi coordinates; see Eq. (9) in the paper. Red color shows lobes of the wavefunction with a different sign. The contours denote the potential. Dashed contours correspond to negative values. The diabaticization is done by solving a differential equation for the rotation matrix.<sup>4</sup> Only the first 10 states are included in the diabaticization procedure and the coupling due to the  $R^{-2}$  term in the kinetic energy is omitted.

#### iv. Kinetic energy release spectra

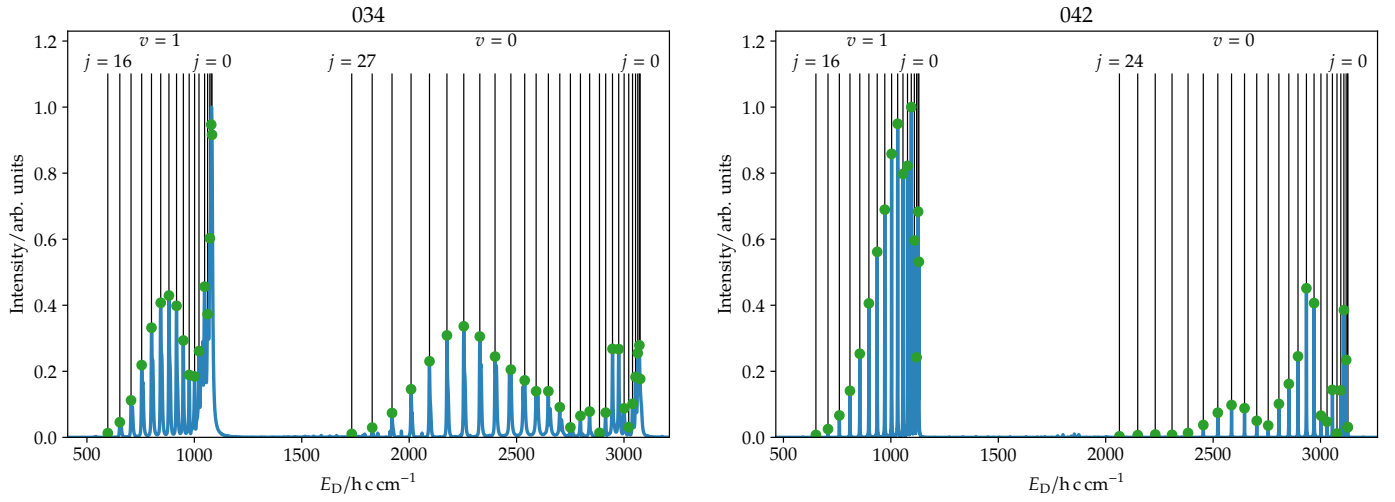

Figure iv: Kinetic energy release spectra of the D atom for resonances (0,3,4) (left) and (0,4,2) (right) using the WKS PES.<sup>1,2</sup> The vertical lines show the assignment of the quantum numbers of the asymptotic CO fragment. The first upper line shows the CO stretch quantum number  $v$  and the second line the minimal and maximal shown rotational/bend quantum number  $j$ . The distributions are scaled such that the maximal value is 1.

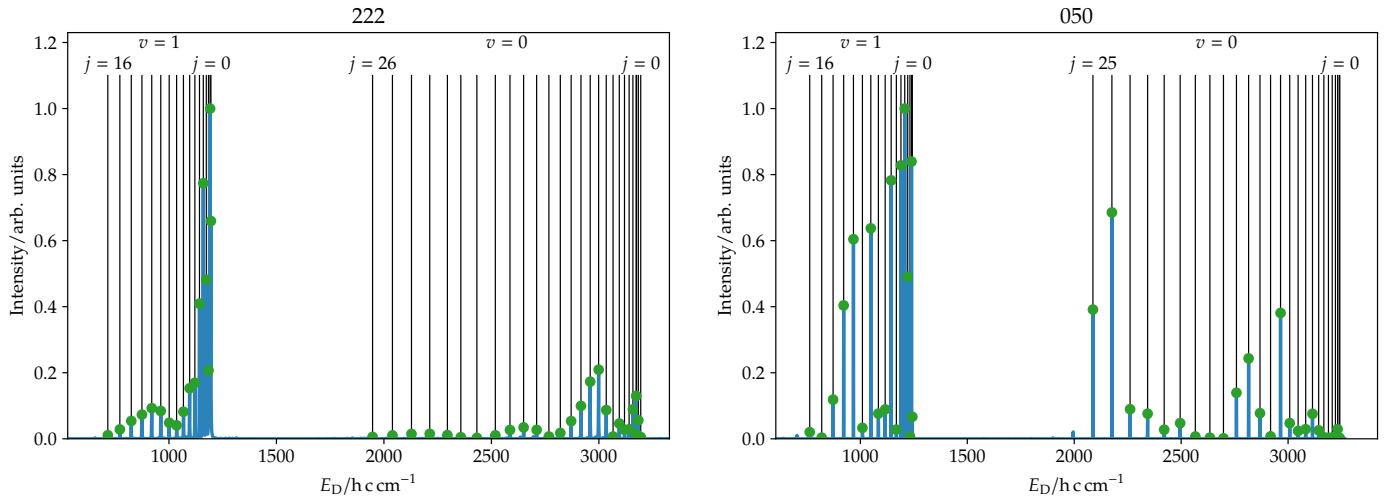

Figure v: Same as Figure iv but with resonances (2,2,2) (left) and (0,5,0) (right).

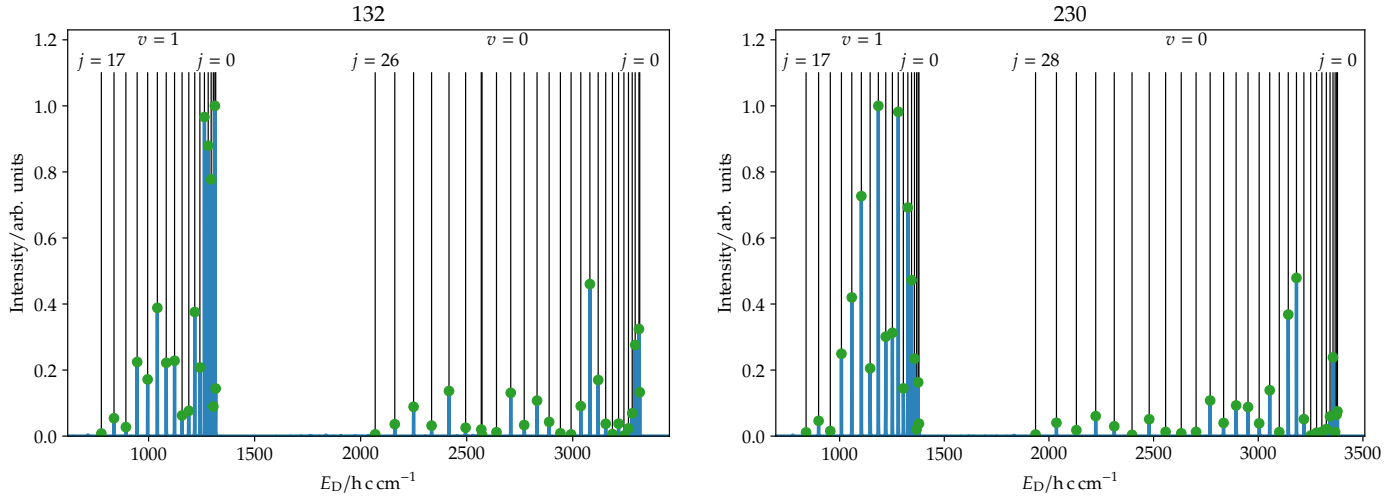

Figure vi: Same as Figure iv but with resonances (1,3,2) (left) and (2,3,0) (right).

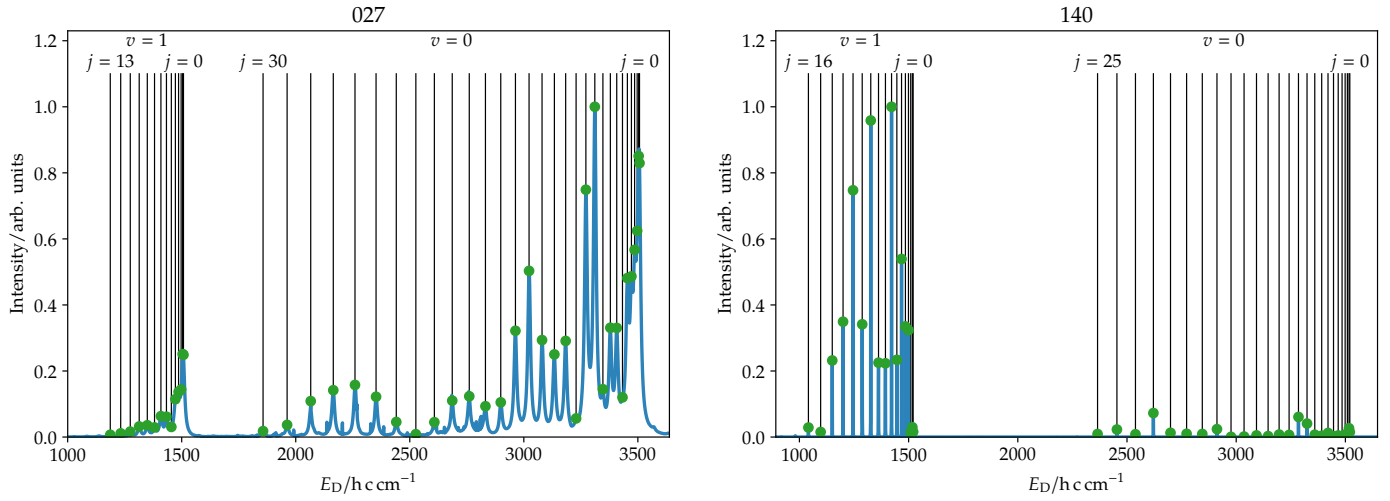

Figure vii: Same as Figure iv but with resonances (0,2,7) (left) and (1,4,0) (right).

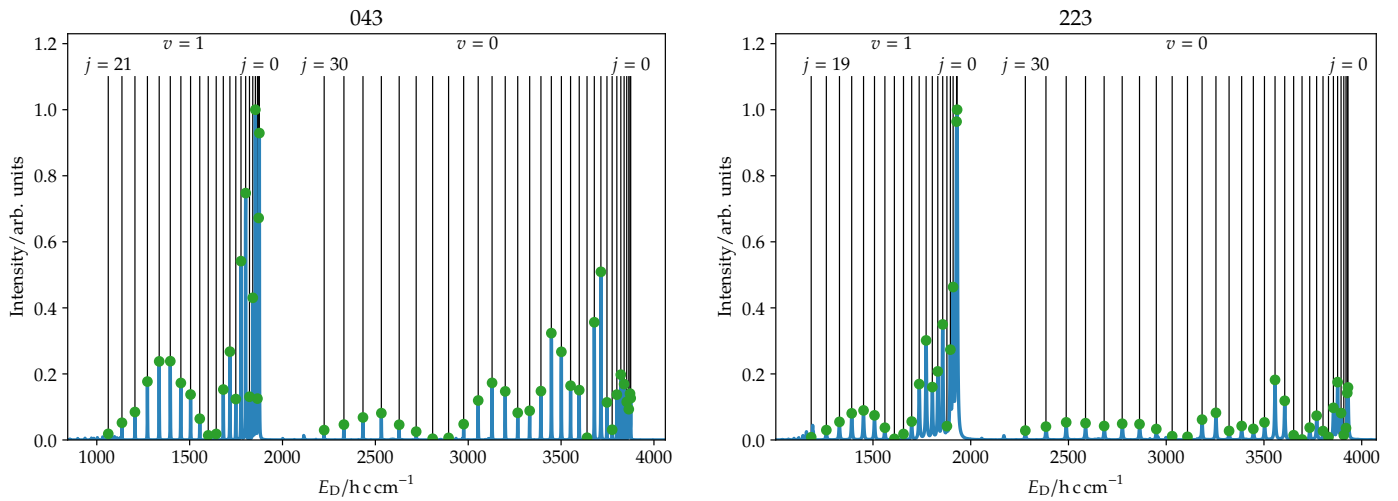

Figure viii: Same as Figure iv but with resonances (0,4,3) (left) and (2,2,3) (right).

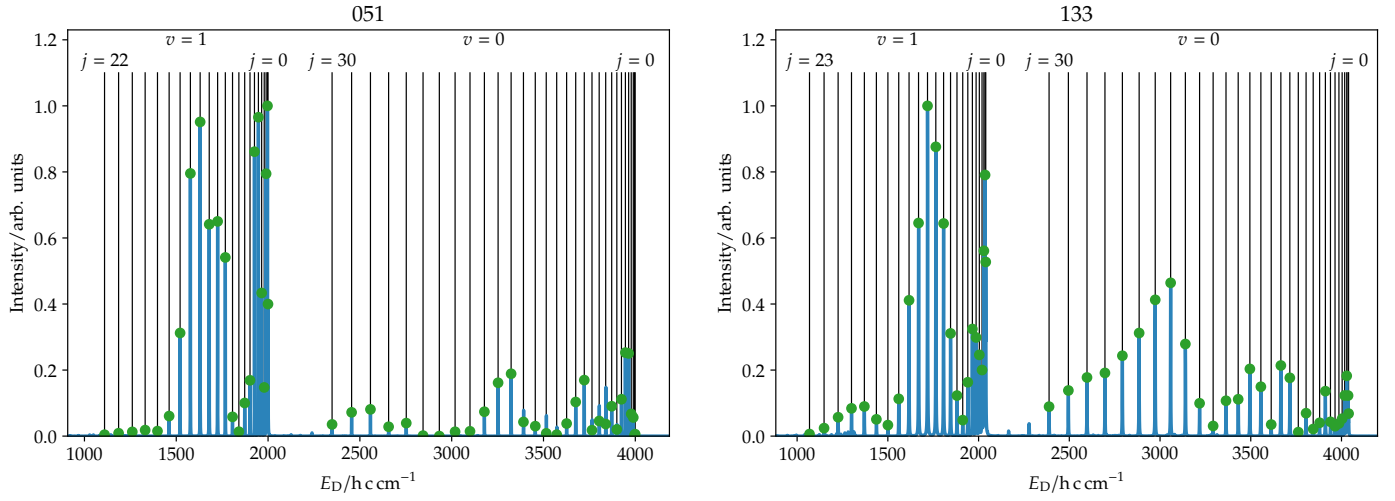

Figure ix: Same as Figure iv but with resonances (0,5,1) (left) and (1,3,3) (right).

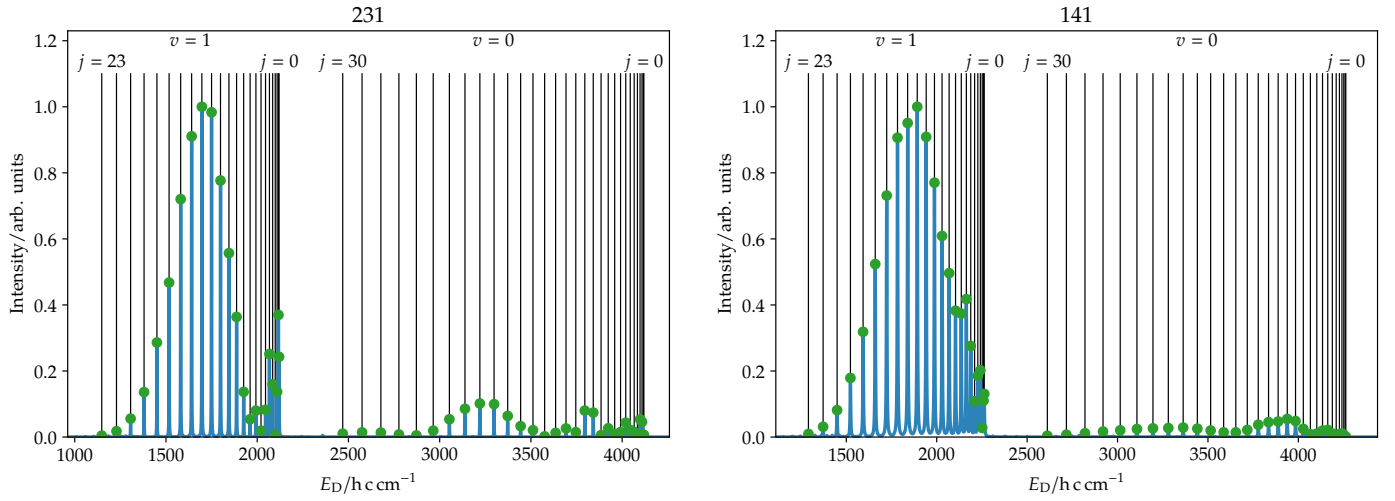

Figure x: Same as Figure iv but with resonances (2,3,1) (left) and (1,4,1) (right).

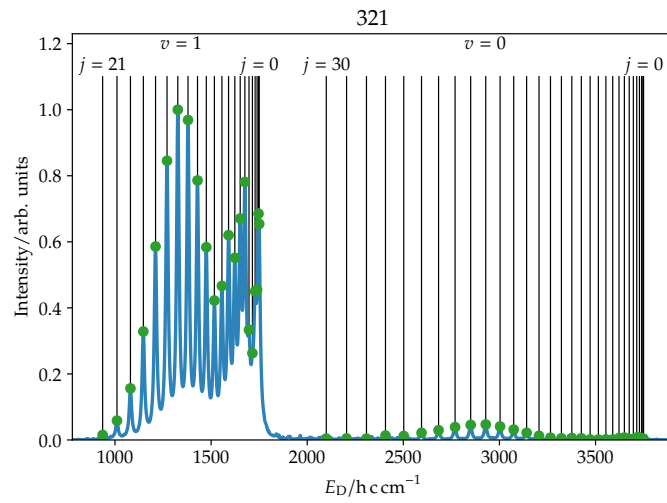

Figure xi: Same as Figure iv but with resonance (3,2,1).

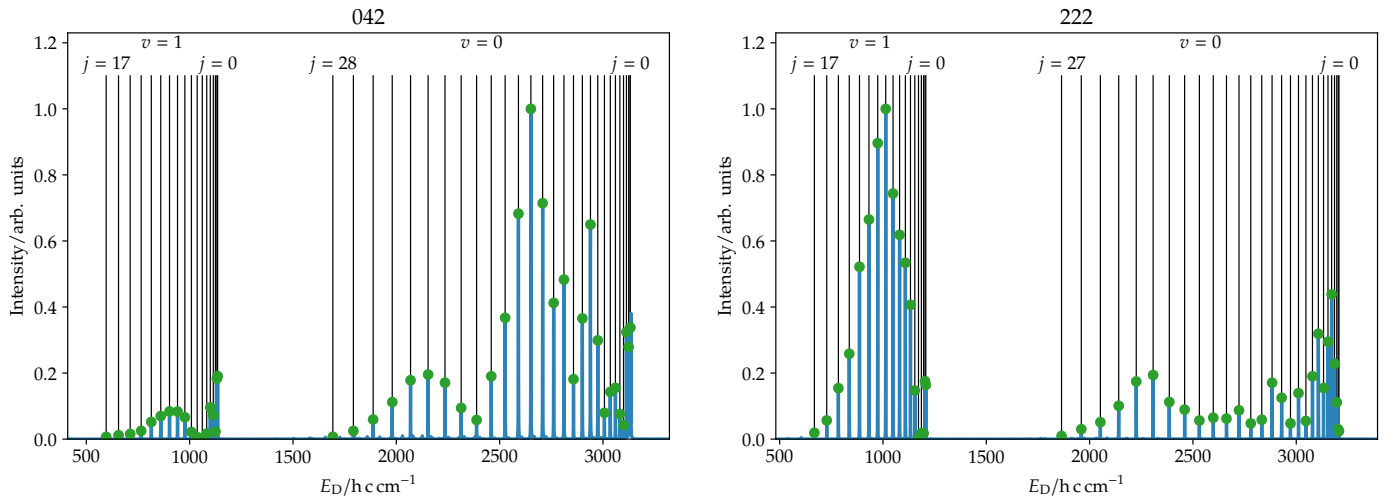

Figure xii: Same as Figure iv but for resonances (0,4,2) (left) and (2,2,2) (right) using the SAG PES.<sup>3</sup>

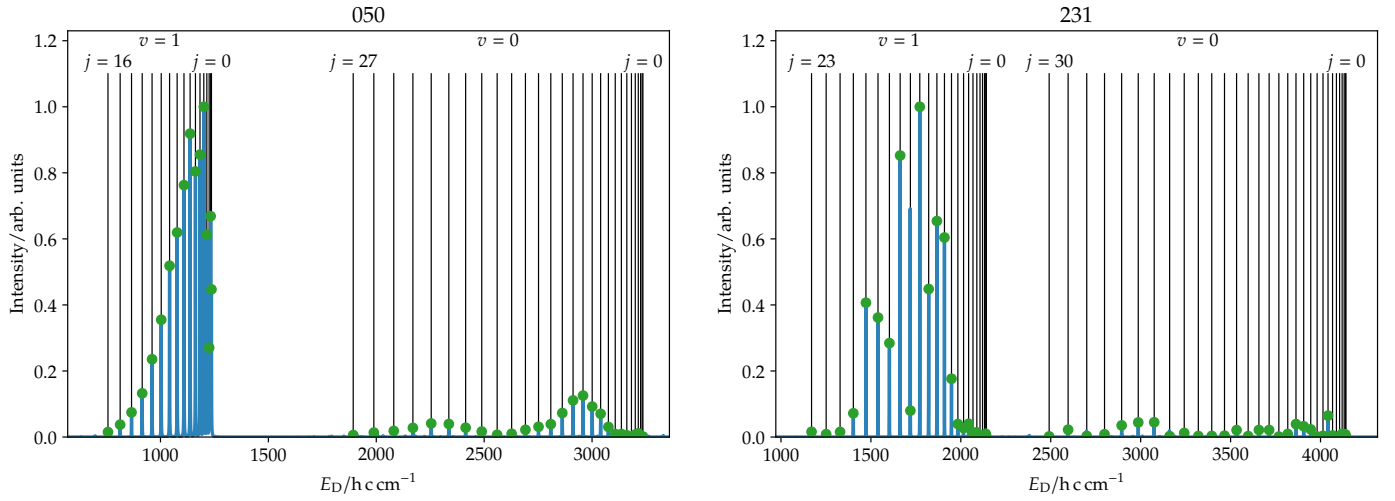

Figure xiii: Same as Figure iv but for resonances (0,5,0) (left) and (2,3,1) (right) using the SAG PES.<sup>3</sup>

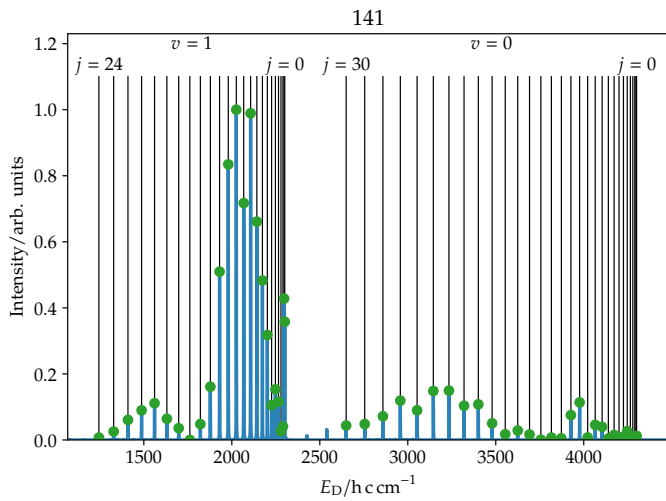

Figure xiv: Same as Figure iv but for resonance (1,4,1) using the SAG PES.<sup>3</sup>

## v. Rovibrational CO product distributions

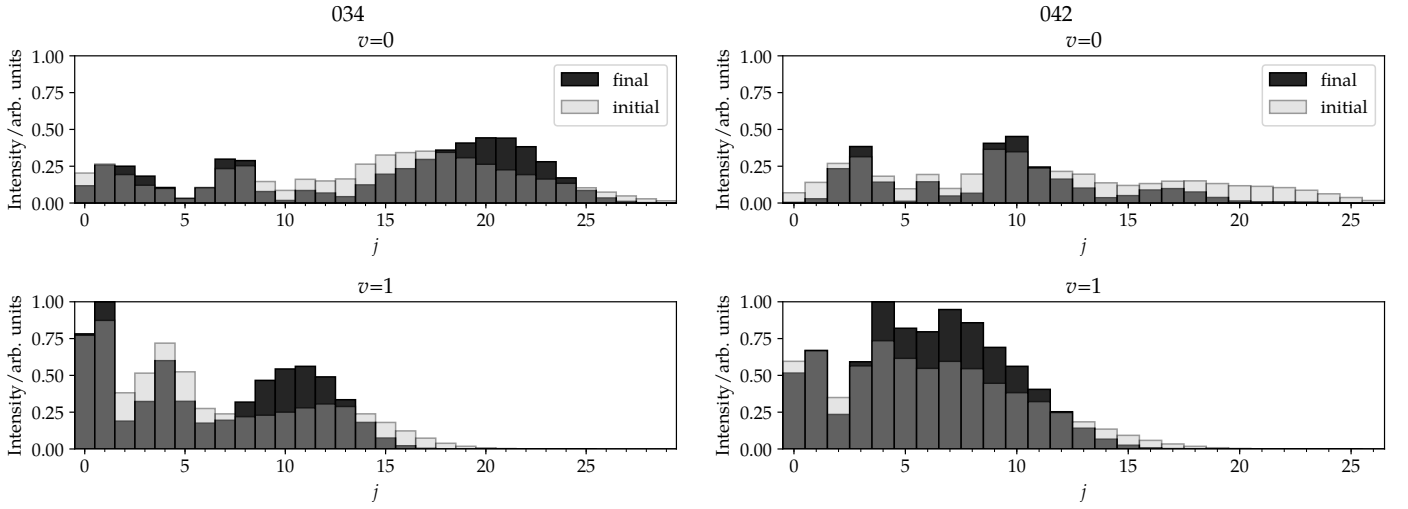

Figure xv: Asymptotic CO quantum-number resolved distributions for resonances (0,3,4) (left) and (0,4,2) (right) using the WKS PES.<sup>1,2</sup> The upper (lower) panels show the distributions for stretch quantum number  $v = 0$  ( $v = 1$ ) versus different rotational quantum numbers  $j$  of the asymptotic CO fragment. The distributions are scaled such that the maximal value is 1. The darker bars show the distributions for the final wavepacket,  $|\Psi(t \rightarrow \infty)\rangle$ . The brighter bars show the distributions for the *initial* wavepacket,  $|\Psi(t = 0)\rangle$ , in the asymptotic region.

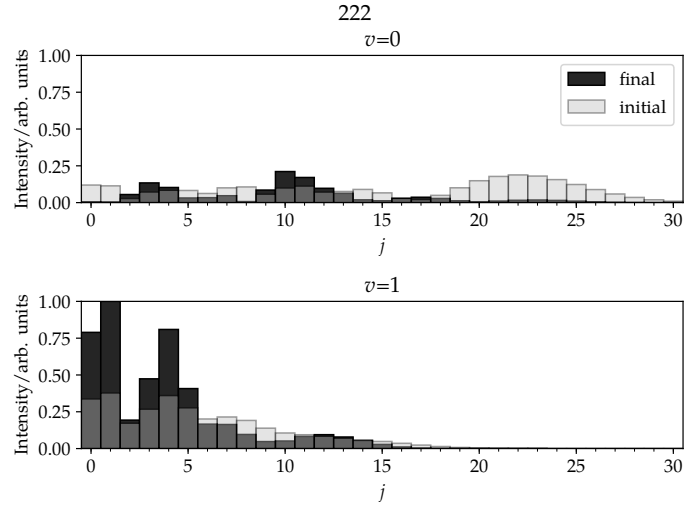

Figure xvi: Same as Figure xv but with resonance (2,2,2).

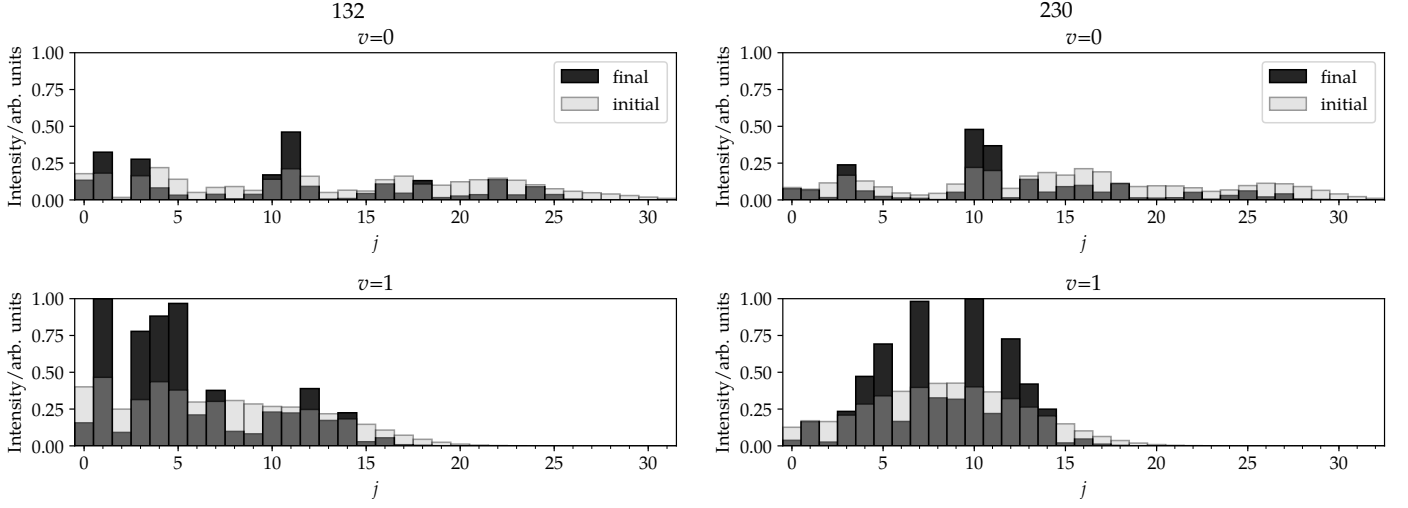

Figure xvii: Same as Figure xv but with resonances (1,3,2) (left) and (2,3,0) (right).

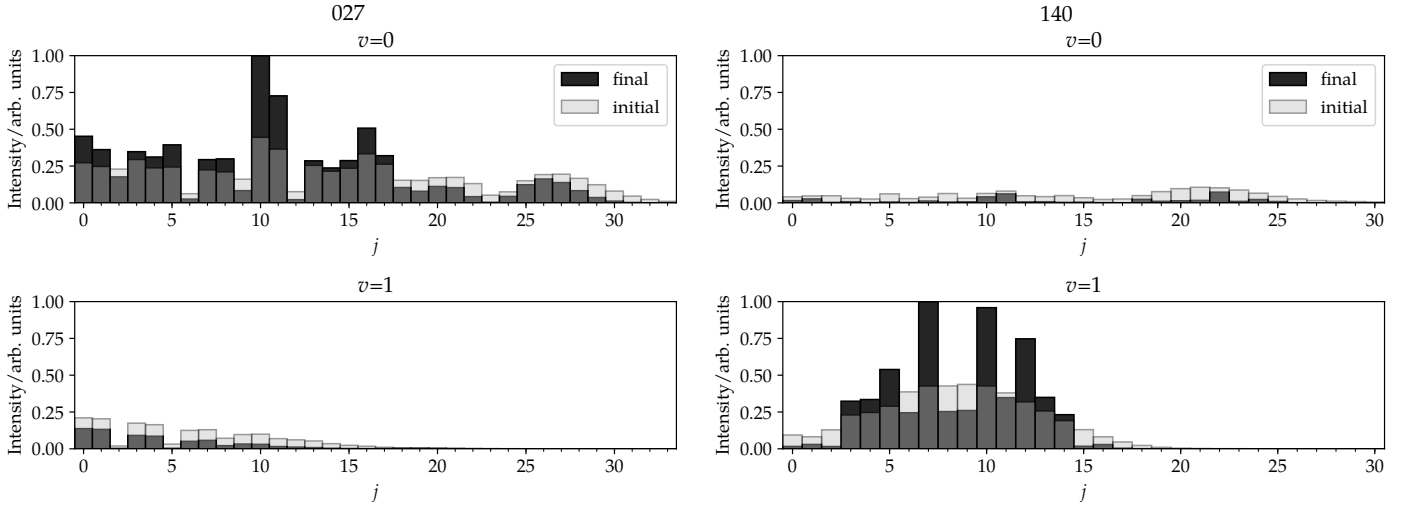

Figure xviii: Same as Figure xv but with resonances (0,2,7) (left) and (1,4,0) (right).

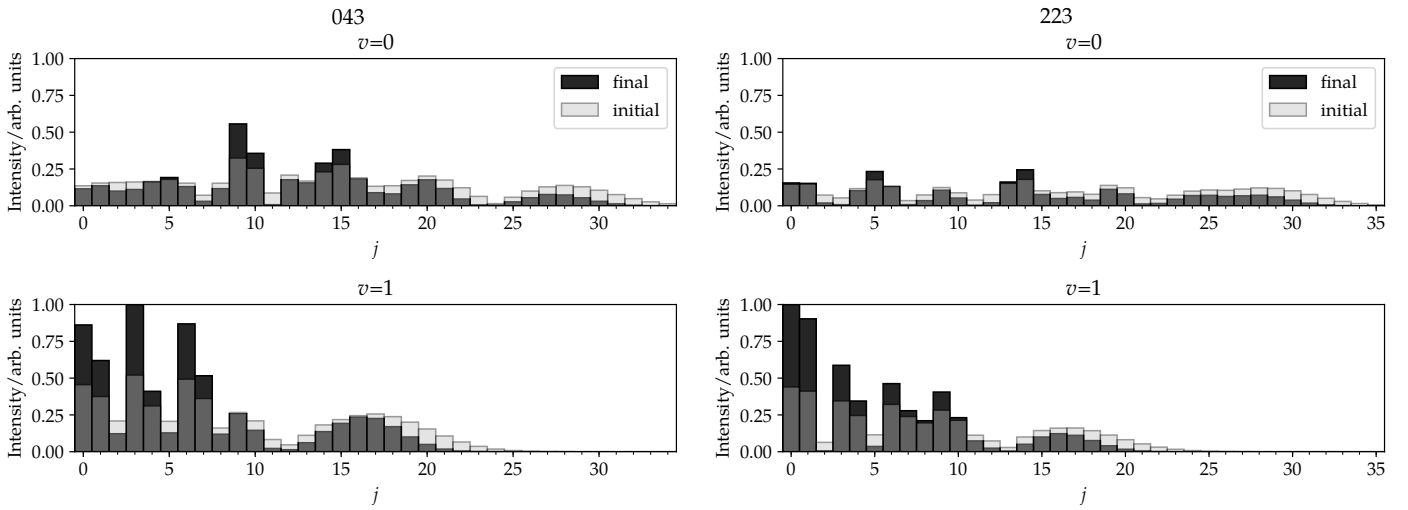

Figure xix: Same as Figure xv but with resonances (0,4,3) (left) and (2,2,3) (right).

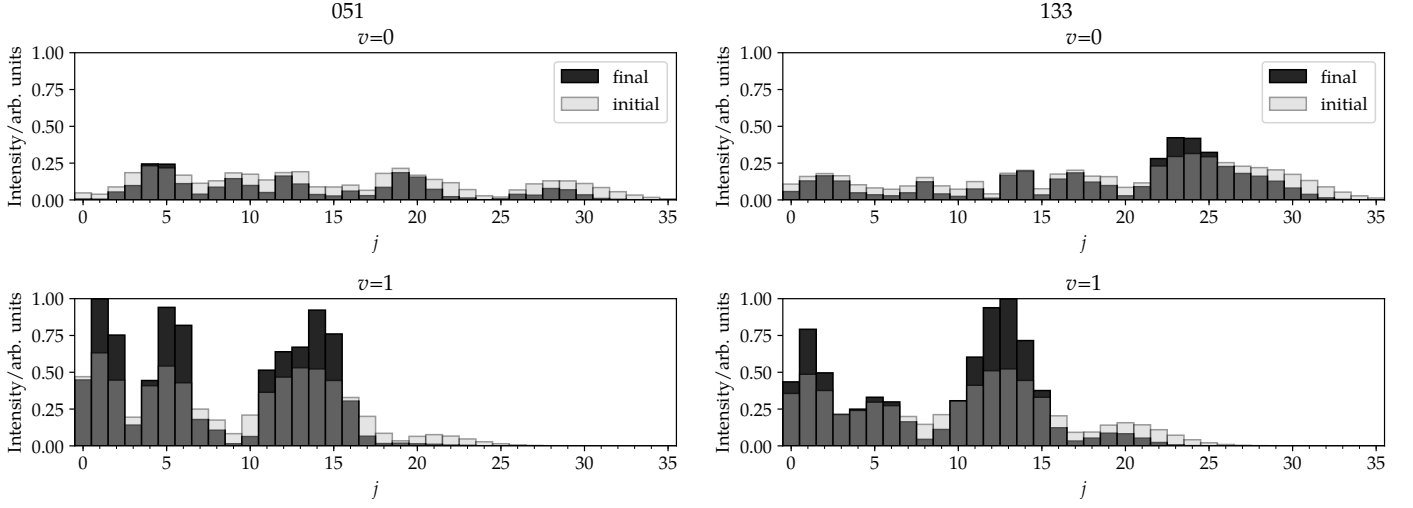

Figure xx: Same as Figure xv but with resonances (0,5,1) (left) and (1,3,3) (right).

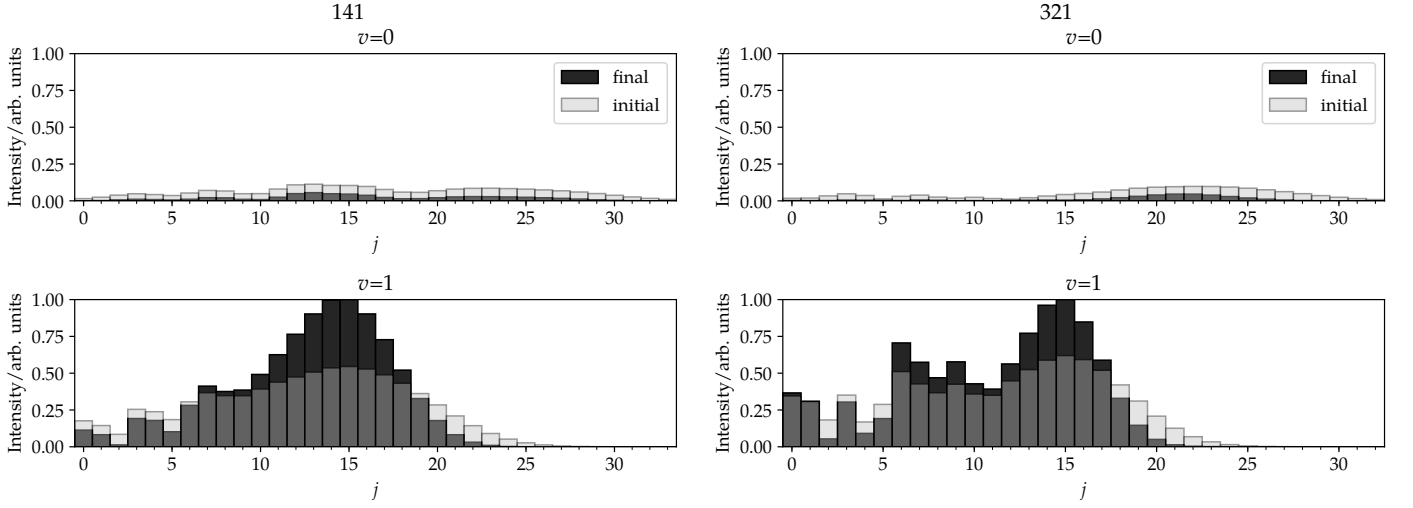

Figure xxi: Same as Figure xv but with resonances (1,4,1) (left) and (3,2,1) (right).

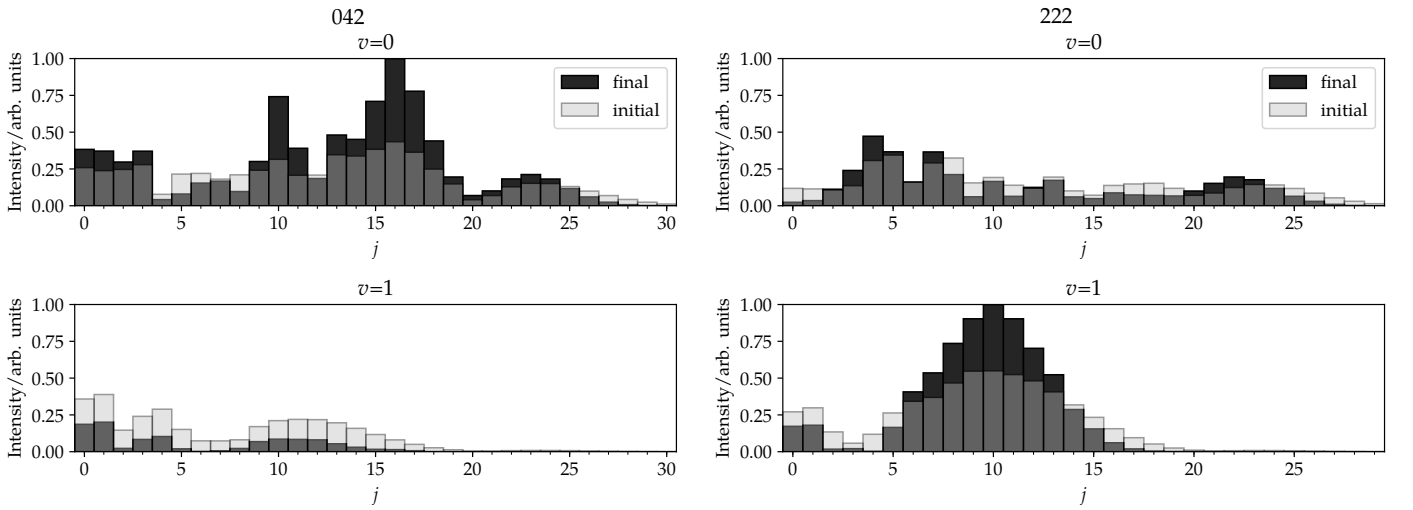

Figure xxii: Same as Figure xv but for resonances (0,4,2) (left) and (2,2,2) (right) using the SAG PES.<sup>3</sup>

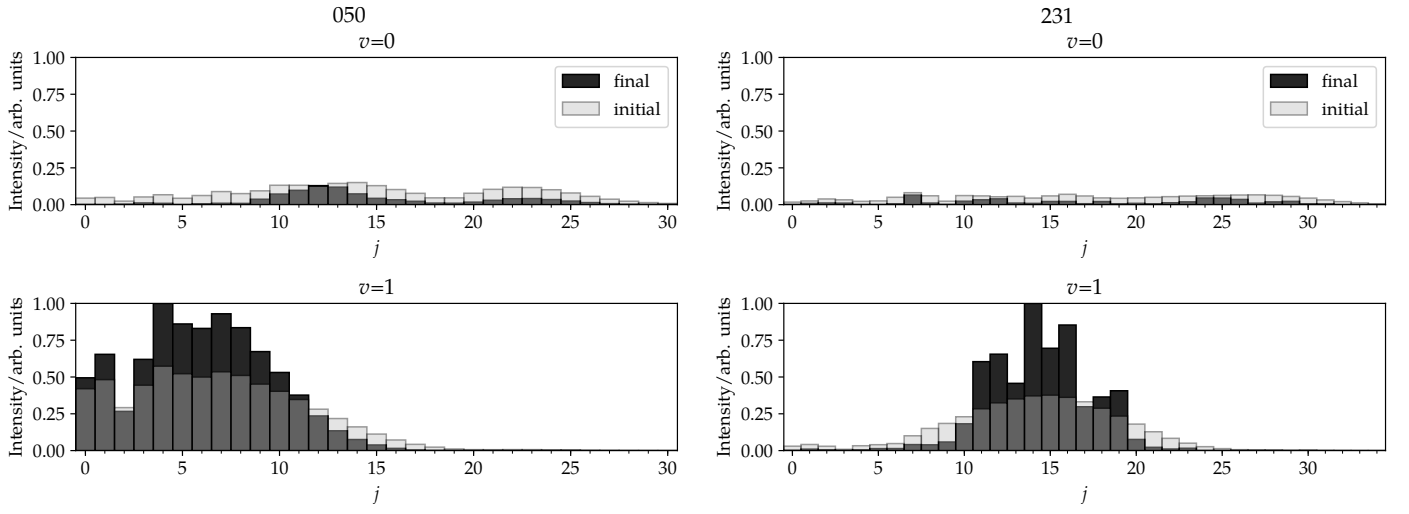

Figure xxiii: Same as Figure xv but for resonances (0,5,0) (left) and (2,3,1) (right) using the SAG PES.<sup>3</sup>

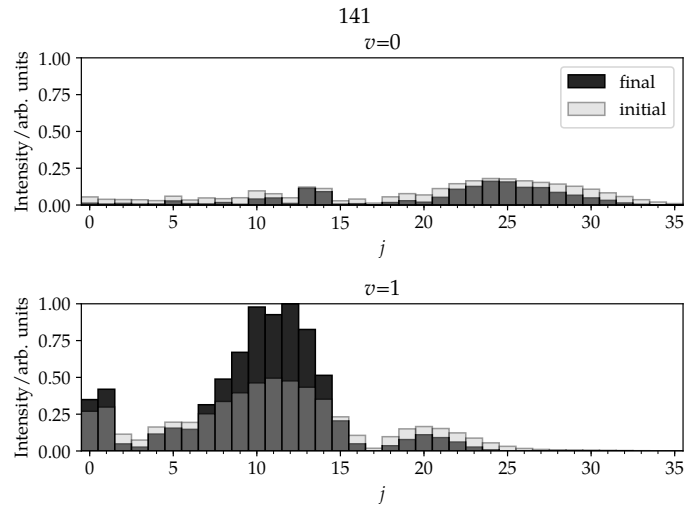

Figure xxiv: Same as Figure xv but for resonance (1,4,1) using the SAG PES.<sup>3</sup>

## References

- <sup>1</sup> Werner, H.-J.; Bauer, C.; Rosmus, P.; Keller, H.-M.; Stumpf, M.; Schinke, R. The Unimolecular Dissociation of HCO: I. Oscillations of Pure CO Stretching Resonance Widths. *J. Chem. Phys.* **1995**, *102*, 3593–3611.
- <sup>2</sup> Keller, H.-M.; Floethmann, H.; Dobbyn, A. J.; Schinke, R.; Werner, H.-J.; Bauer, C.; Rosmus, P. The Unimolecular Dissociation of HCO. II. Comparison of Calculated Resonance Energies and Widths with High-resolution Spectroscopic Data. *J. Chem. Phys.* **1996**, *105*, 4983–5004.
- <sup>3</sup> Song, L.; van der Avoird, A.; Groenenboom, G. C. Three-Dimensional Ab Initio Potential Energy Surface for H-CO(X2A). *J. Phys. Chem. A* **2013**, *117*, 7571–7579.
- <sup>4</sup> Baer, M. Adiabatic and Diabatic Representations for Atom-Molecule Collisions: Treatment of the Collinear Arrangement. *Chem. Phys. Lett.* **1975**, *35*, 112–118.
- <sup>5</sup> Pacher, T.; Köppel, H.; Cederbaum, L. S. Quasidiabatic States from Ab Initio Calculations by Block Diagonalization of the Electronic Hamiltonian: Use of Frozen Orbitals. *J. Chem. Phys.* **1991**, *95*, 6668–6680.
- <sup>6</sup> Simah, D.; Hartke, B.; Werner, H.-J. Photodissociation Dynamics of H<sub>2</sub>S on New Coupled *Ab Initio* Potential Energy Surfaces. *J. Chem. Phys.* **1999**, *111*, 4523–4534.
- <sup>7</sup> Mitrushenkov, A. O.; Palmieri, P.; Puzzarini, C.; Tarroni, R. Numerical Techniques for the Evaluation of Non-Adiabatic Interactions and the Generation of Quasi-Diabatic Potential Energy Surfaces Using Configuration Interaction Methods. *Mol. Phys.* **2000**, *98*, 1677–1690.
- <sup>8</sup> Köppel, H.; Domcke, W.; Cederbaum, L. S. Multimode Molecular Dynamics Beyond the Born-Oppenheimer Approximation. *Adv. Chem. Phys.* **57**, 59–246.
- <sup>9</sup> Wittenbrink, N.; Venghaus, F.; Williams, D.; Eisfeld, W. A New Approach for the Development of Diabatic Potential Energy Surfaces: Hybrid Block-Diagonalization and Diabatization by Ansatz. *J. Chem. Phys.* **2016**, *145*, 184108.
- <sup>10</sup> Esry, B. D.; Sadeghpour, H. R. Split Diabatic Representation. *Phys. Rev. A* **2003**, *68*.
